# Supplementary material for: Uncertainty-Guided Enhancement on Driving Perception System via Foundation Models
Source: arXiv:2410.01144 source file (2024-10-02)
Supplement: Supplementary file 1 [file A-appendix.tex]

\newpage
\appendix

\onecolumn
